# Supplementary material for: On Learning Closed-Loop Probabilistic Multi-Agent Simulator
Source: arXiv:2508.00384 source file (2025-08-01)
Supplement: Supplementary file 1 [file X_suppl.tex]

\section*{Appendix}
\label{sec: Appendix}

\subsection{Synchronous Decision-Making}
\label{subsec: appendix-synchronous}

In this paper, the proposed model NeVA poses a strong assumption that agents in a traffic scenario make decisions at the same time, reflected by the synchronous sampling of latent variables within the autoregressive sampling. However, agents in real-world traffic scenarios make decisions asynchronously due to the heterogeneity in their intentions and driving behaviors. For instance, as illustrated in Figure~\ref{fig: async-decision}, two agents are making decisions in consecutive patch predictions. In NeVA, we assume they make decisions simultaneously at the end of the first patch. In reality, if agent $1$ were making a turn and agent $2$ was following agent $1$, agent $2$ would decide after observing the agent's action $1$, and the duration of taking the action would be shorter. As a result, the next-patch prediction in NeVA can lead to reduced realism in the simulation.

\begin{figure}[!ht]
    \centering
    \includegraphics[width=\linewidth]{img/suppl/async_decision.png}
    \caption{Illustration of the asynchronous decision-making by two agents in consecutive patch predictions.}
    \label{fig: async-decision}
\end{figure}

An easy way to address this issue is to reduce the patch size. Suppose we denote the state of agent $i$ at time $t$ by $\boldsymbol{x}_{t}^{(i)}$, its action by $u_{t}^{(i)}$, and the continuous dynamics of the agent by $f_{i}(x,u)$, then the trajectory of agent $i$ in the next-patch prediction with step size $\tau$ is given by
\begin{equation}
    x_{t+\tau,\text{sync}}^{(i)} = x_{t}^{(i)} + \int_{t}^{t+\tau}f_{i}(x_{s}^{(i)},u_{\tau}^{(i)})ds.
\end{equation}
Suppose in the corresponding asynchronous decision-making, agent $i$ makes its decision after $\delta_{t}^{(i)}$ time steps, where $0\leq\delta_{t}^{(i)}\leq\tau$. The trajectory of agent $i$ in the next-patch prediction is given by
\begin{equation}
    x_{t+\tau,\text{async}}^{(i)} = x_{t}^{(i)} + \int_{t}^{t+\delta_{t}^{(i)}}f_{i}(x_{s}^{(i)},u_{\delta}^{(i)})ds.
\end{equation}
According to Lipschitz continuity, the difference between the two trajectories is bounded by a constant $K_{i}$:
\begin{equation}
    \begin{aligned}
        \left\|\Delta{x_{t+\tau}^{(i)}}\right\|&\leq K_{i}\left\|\int_{t+\delta_{t}^{(i)}}^{t+\tau}f_{i}(x_{s}^{(i)},u_{\tau}^{(i)})ds\right\| \\
        &\leq K_{i}\int_{t}^{t+\tau}\left\|x_{t+s,\text{sync}}^{(i)}-x_{t+s,\text{async}}^{(i)}\right\|ds \\
        &\quad + K_{i}\int_{t}^{t+\tau}\left\|u_{\tau}^{(i)} - u_{\delta}^{(i)}\right\|ds.
    \end{aligned}
\end{equation}
For the same agent, it is reasonable to assume that the difference in decided actions is bounded by a constant $\left\|u_{\tau}^{(i)}-u_{\delta}^{(i)}\right\|\leq M$. Based on Gr\"onwall's inequality, the difference between the trajectories is upper-bounded by
\begin{equation}
    \left\|\Delta{x_{t+\tau}^{(i)}}\right\|\leq K_{i}M\tau e^{K_{i}\tau}.
\end{equation}
Therefore, with reducing step size $\tau$, the difference is asymptotically zero: $\lim_{\tau\to 0}\left\|\Delta{x_{t+\tau}^{(i)}}\right\|=0$. The trade-off here is that reducing the step size leads to an increased number of sampling steps, which can be computationally expensive. Therefore, in our experiments, we set $\tau=10$ to balance the realism and computation efficiency.

% ------------------------------------------------------------------------

\subsection{Conditional and Marginal Gaussian}
\label{subsec: appendix-conditional-marginal-gauss}

NeVA uses a linear layer to model the dependencies between the latent variable $h^{(n)}_{d,k}$ and the future observation $\boldsymbol{o}^{(n)}_{d,k}$ of agent $n$ at patch $d$, which writes
\begin{equation}
    \boldsymbol{o}^{(n)}_{k} = Ah^{(n)}_{d,k} + b + \varepsilon, \quad \varepsilon\sim\mathcal{N}(0,\boldsymbol{L}).
\end{equation}
This linear emission structure is beneficial for both training and sampling since it yields closed-form analytical solutions for the posterior distribution $p(h^{(n)}_{dk}|\boldsymbol{o}^{(n)}_{dk})$ and the marginal distribution of $p(\boldsymbol{o}^{(n)}_{dk})$. The former can be used in the recognition model to investigate the temporal dynamics of different agents, while the latter is the key to our training and sampling procedures. This section provides a detailed derivation of the conditional and marginal Gaussian distributions in the linear Gaussian model.

For convenience, we abuse the notation by dropping the superscripts and denote the mean vector and covariance matrix of $p(h_{dk})$ by $\mu$ and $\boldsymbol{\Sigma}$, and the covariance matrix in $p(\boldsymbol{o}_{dk}|h_{dk})$ by $\boldsymbol{L}$. The logarithm of marginal and conditional emission density to a constant is given by
\begin{equation}
    \begin{aligned}
        \log p(h_{dk}) &= -\frac{1}{2}(h_{dk}-\boldsymbol{\mu})^{\intercal}\boldsymbol{\Sigma}^{-1}(h_{dk}-\boldsymbol{\mu}), \\
        \log p(\boldsymbol{o}_{dk}|h_{dk}) &= -\frac{1}{2}(\boldsymbol{o}_{dk}-\boldsymbol{f}_{dk})^{\intercal}\boldsymbol{L}^{-1}(\boldsymbol{o}_{dk}-\boldsymbol{f}_{dk}), \\
    \end{aligned}
\end{equation}
where $\boldsymbol{f}_{dk}=Ah_{dk}+b$. Hence, the logarithm of the joint density is given by
\begin{equation}
    \begin{aligned}
        \log p(h_{dk},\boldsymbol{o}_{dk}) &= \log p(h_{dk}) + \log p(\boldsymbol{o}_{dk}|h_{dk}) \\
        &= -\frac{1}{2}\bigl[h_{dk}^{\intercal}(\boldsymbol{\Sigma}^{-1} + A^{\intercal}\boldsymbol{L}^{-1}A)h_{dk} \\
        &\quad\quad\quad - 2h_{dk}^{\intercal}A^{\intercal}\boldsymbol{L}^{-1}\boldsymbol{o}_{dk} \\
        &\quad\quad\quad + \boldsymbol{y}_{dk}^{\intercal}A\boldsymbol{o}_{dk}\bigr] + C \\
        &= -\frac{1}{2}\boldsymbol{v}\boldsymbol{P}\boldsymbol{v} + C
    \end{aligned}
    \label{eq: joint-normal-expansion}
\end{equation}
where $C$ is a constant independent of the joint vector $\boldsymbol{v} = [h_{dk}, \boldsymbol{o}_{dk}]^{\intercal}$. From the formulation, we can assert that the joint distribution $p(\boldsymbol{v})$ is a Gaussian distribution with a precision matrix given by
\begin{equation}
    \boldsymbol{P} = \begin{pmatrix}\boldsymbol{\Sigma}^{-1} + A^{\intercal}\boldsymbol{L}^{-1}A & -A^{\intercal}\boldsymbol{L}^{-1} \\ -\boldsymbol{L}^{-1}A & \boldsymbol{L}^{-1}\end{pmatrix}.
    \label{eq: joint-precision}
\end{equation}
Meanwhile, we further extract the linear terms from $C$ in the expansion, which writes
\begin{equation}
    \begin{aligned}
    &\boldsymbol{\mu}^{\intercal}\boldsymbol{\Sigma}^{-1}h_{dk} + b^{\intercal}\boldsymbol{L}^{-1}Ah_{dk} + b^{\intercal}\boldsymbol{L}^{-1}\boldsymbol{o}_{dk} \\
    =& \begin{pmatrix}\boldsymbol{\mu}^{\intercal}\boldsymbol{\Sigma}^{-1} + b^{\intercal}\boldsymbol{L}^{-1}A \\ b^{\intercal}\boldsymbol{L}^{-1}\end{pmatrix}\boldsymbol{v}.
    \end{aligned}
\end{equation}
We can derive the mean of the joint distribution by completing the square in log density:
\begin{equation}
    \mathbb{E}[\boldsymbol{v}] = \boldsymbol{P}^{-1}\begin{pmatrix}\boldsymbol{\mu}^{\intercal}\boldsymbol{\Sigma}^{-1} + b^{\intercal}\boldsymbol{L}^{-1}A \\ b^{\intercal}\boldsymbol{L}^{-1}\end{pmatrix} = \begin{pmatrix}
        \boldsymbol{\mu} \\ A\boldsymbol{\mu} + b
    \end{pmatrix}
    \label{eq: joint-mean}
\end{equation}

Making use of the results from equation (\ref{eq: joint-precision}) and (\ref{eq: joint-mean}), we can obtain the means and covariance matrices in the marginal distribution of $y_{k}$:
\begin{equation}
    p(\boldsymbol{o}_{dk})\sim\mathcal{N}(A\boldsymbol{\mu} + b, \boldsymbol{L} + A\boldsymbol{\Sigma}A^{\intercal}),
    \label{eq: marginal-emission}
\end{equation}
and in the conditional posterior distribution of $s_{k}$:
\begin{equation}
    p(h_{dk}|\boldsymbol{o}_{dk})\sim\mathcal{N}\left(\boldsymbol{S}\left\{A^{\intercal}\boldsymbol{L}^{-1}(\boldsymbol{o}_{dk}-b)+\boldsymbol{\Sigma}^{-1}\boldsymbol{\mu}\right\},\boldsymbol{S}\right),
    \label{eq: linear-gaussian-posterior}
\end{equation}
where $\boldsymbol{S}=(\boldsymbol{\Sigma}^{-1}+A^{\intercal}\boldsymbol{L}^{-1}A)^{-1}$. The derived property is widely used in building linear Gaussian models~\cite{6790691}.

\begin{figure*}[!htbp]
    \centering
    \includegraphics[width=\textwidth]{img/suppl/viz_intersection.png}
    \caption{\textbf{Visulization of representive cases with signalized intersections.}}
    \label{fig: viz-intersection}
\end{figure*}
\begin{figure*}[!htbp]
    \centering
    \includegraphics[width=\textwidth]{img/suppl/viz_segment.png}
    \caption{\textbf{Visuliazation of representative cases on road segments.}}
    \label{fig: viz-segment}
\end{figure*}

% ------------------------------------------------------------------------

\subsection{Variational Inference}
\label{subsec: appendix-vi}
This section details the variational inference algorithm for training the NeVA model. Following~\cite{doi:10.1080/01621459.2017.1285773}, the training objective is derived by minimizing the Kullback-Leibler (KL) divergence between the variational and actual posterior distributions:
\begin{equation}
    \begin{aligned}
        \mathcal{L}(\theta;n,k) =& D_{\text{KL}}\left[\check{p}(\pi,\boldsymbol{z})\big\|\hat{p}(\pi,\boldsymbol{z};\theta)\right] \\
        =& \mathbb{E}_{\check{p}(\pi, \boldsymbol{z})}\log\left[\prod\limits_{n=1}^{N}\frac{\check{p}(z_{n}\mid\pi)\check{p}(\pi)}{\hat{p}(\boldsymbol{o}^{(n)}|z_{n};\theta)\hat{p}(z_{n},\pi;\theta)} + \text{const}\right] \\
        =& -\sum\limits_{n=1}^{N}\sum\limits_{d=1}^{D}\mathbb{E}_{\check{p}(z_{n})}\log\hat{p}(\boldsymbol{o}_{d+1}^{(n)}|\boldsymbol{s}_{d},\mathcal{M},z_{n};\theta) \\
        & + \sum\limits_{n=1}^{N}\mathbb{E}_{\check{p}(\pi)}D_{\text{KL}}\bigl[\check{p}(z_{n})\big\|\hat{p}(z_{n}|\pi;\theta)\bigr] \\
        & + D_{\text{KL}}\bigl[\check{p}(\pi)\big\|\hat{p}(\pi;\theta)\bigr],
    \end{aligned}
\end{equation}
where $\text{const}$ is a constant independent of model parameters $\theta$. Minimizing the KL divergence is equivalent to maximizing the lower bound of the conditional log-likelihood $\log\hat{p}(\boldsymbol{o}|\boldsymbol{s},\mathcal{M})$ with respect to $\theta$.

Suppose we denote the probability in the variational Categorical distribution $\check{p}(z_{n})$ by $\phi_{n}$, and the concentration in the variational Dirichlet distribution $\check{p}(\pi)$ by $\alpha^{\prime}$, we can calculate the optimal $\phi_{n}$ by taking the derivatives of the loss function with respect to $\phi_{n}$:
\begin{equation}
    \frac{\partial\mathcal{L}}{\partial\phi_{nk}} = -\sum\limits_{d=1}^{D}\log\hat{p}(\boldsymbol{o}_{d+1}^{(n)}|z_{n}) + \log\phi_{nk} - \psi(\alpha_{k}^{\prime}) + \psi\left(\sum\limits_{k=1}^{K}\alpha_{k}^{\prime}\right).
\end{equation}
By introducing the Lagrangian term $\sum_{k=1}^{K}\phi_{nk}=1$, the optimal $\phi_{n}$ can be derived as
\begin{equation}
    \phi_{nk}^{\ast} = \text{Softmax}\left(\sum\limits_{d=1}^{D}\log\hat{p}(\boldsymbol{o}_{d+1}^{(n)}|z_{n}) + \psi(\alpha_{k}^{\prime}) - \psi\left(\sum\limits_{k=1}^{K}\alpha_{k}^{\prime}\right)\right).
\end{equation}
Similarly, the optimal $\alpha^{\prime}$ can be derived by taking the derivatives of the loss function with respect to $\alpha_{k}^{\prime}$:
\begin{equation}
    \begin{aligned}
        \frac{\partial\mathcal{L}}{\partial\alpha_{k}^{\prime}} &= \digamma(\alpha_{k}^{\prime})\left(\alpha_{k}+\sum\limits_{n=1}^{N}\phi_{nk}-\alpha^{\prime}_{k}\right) \\
        &\quad - \digamma\left(\sum\limits_{k=1}^{K}\alpha_{k}^{\prime}\right)\left(\alpha_{j} + \sum\limits_{n=1}^{N}\phi_{nk}-\alpha_{k}^{\prime}\right),
    \end{aligned}
\end{equation}
where $\digamma(\cdot)$ is the derivative of the digamma function. By setting the derivatives to zero, the optimal $\alpha^{\prime}$ writes
\begin{equation}
    \alpha_{k}^{\prime\ast} = \alpha_{k} + \sum\limits_{n=1}^{N}\phi_{nk}.
\end{equation}

Herein, the problem of optimizing the objective function is that the optimal variational parameters interleave as functions of each other. To address this issue, we propose to use the variational expectation maximization (EM) algorithm. Specifically, we first evaluate the optimal $\phi_{n}$ by setting $\alpha^{\prime}$ as the current value of $\alpha$. Then, we evaluate the optimal $\alpha^{\prime}$, we set $\phi_{n}$ to be the current value of $\phi_{n}$. Finally, we optimize $\theta$ by applying gradient descent on the loss function $\mathcal{L}(\theta;n,k)$ with evaluated $\phi_{n}$ and $\alpha^{\prime}$ and their gradients detached.

% ------------------------------------------------------------------------
% \section{Additional Implementation Details}
% \label{sec: appendix-implementation}

% ------------------------------------------------------------------------

\subsection{Additional Results in Experiments}
\label{subsec: appedix-results}

In this section, we provide additional visualization of the simulated scenario using the proposed NeVA model. Figure~\ref{fig: viz-intersection} shows cases that involve signalized intersections, where NeVA predicts the reasonable trajectories of agents and learns the lane directions at the entrances. In Figure~\ref{fig: viz-segment}, we visualize cases on other road segments. The predicted trajectories are consistent with the road geometry. The results suggest that NeVA can simulate complicated traffic scenarios with fidelity.
